# Supplementary material for: Spectrum from Defocus: Fast Spectral Imaging with Chromatic Focal Stack
Source: arXiv:2503.20184 source file (2026-02-11)
Supplement: Supplementary file 1 [file X_suppl.tex]

\newcounter{si}
\setcounter{si}{0} % Reset section counter
%section numbering to alphabetical

\newcounter{supfigure}
\setcounter{supfigure}{0}
\newcounter{suptable}
\setcounter{suptable}{0}
\newenvironment{suppfigure}{
     % Use "S" prefix
    \refstepcounter{supfigure} % Automatically increment the supplementary figure counter
    \figure
}{
    \endfigure
}

\newenvironment{suppfigure*}{
     % Use "S" prefix
    \refstepcounter{supfigure} % Automatically increment the supplementary figure counter
    \begin{figure*} % Two-column figure
}{
    \end{figure*}
}

% Define a new environment for supplementary tables
\newenvironment{supptable}[1][]{%
    \refstepcounter{suptable} % Increment the supplementary table counter
     % Use the supplementary table numbering within this environment
    \begin{table}[#1] % Start the table environment with optional positioning
}{
    \end{table}
}
\newenvironment{supptable*}[1][]{%
    \refstepcounter{suptable} % Increment the supplementary table counter
     % Use the supplementary table numbering within this environment
    \begin{table*}[#1] % Start the table environment with optional positioning
}{
    \end{table*}
}

\newcounter{supequation}
\setcounter{supequation}{0}

% Define a new environment for supplementary tables

\clearpage

\setcounter{page}{1}
\maketitlesupplementary

\stepcounter{si}
\section{Lens positions}
\label{sec: lens positions}
SfD leverages the chromatic information resulting from the varying lens positions. To ensure that the chromatic responses corresponding to different lens locations do not overlap too much, we select lens positions that are evenly distributed across the focal-shift range (see \cref{fig:focal_shift_locs}).
\begin{suppfigure*}
    \centering
    \includegraphics[width=\textwidth]{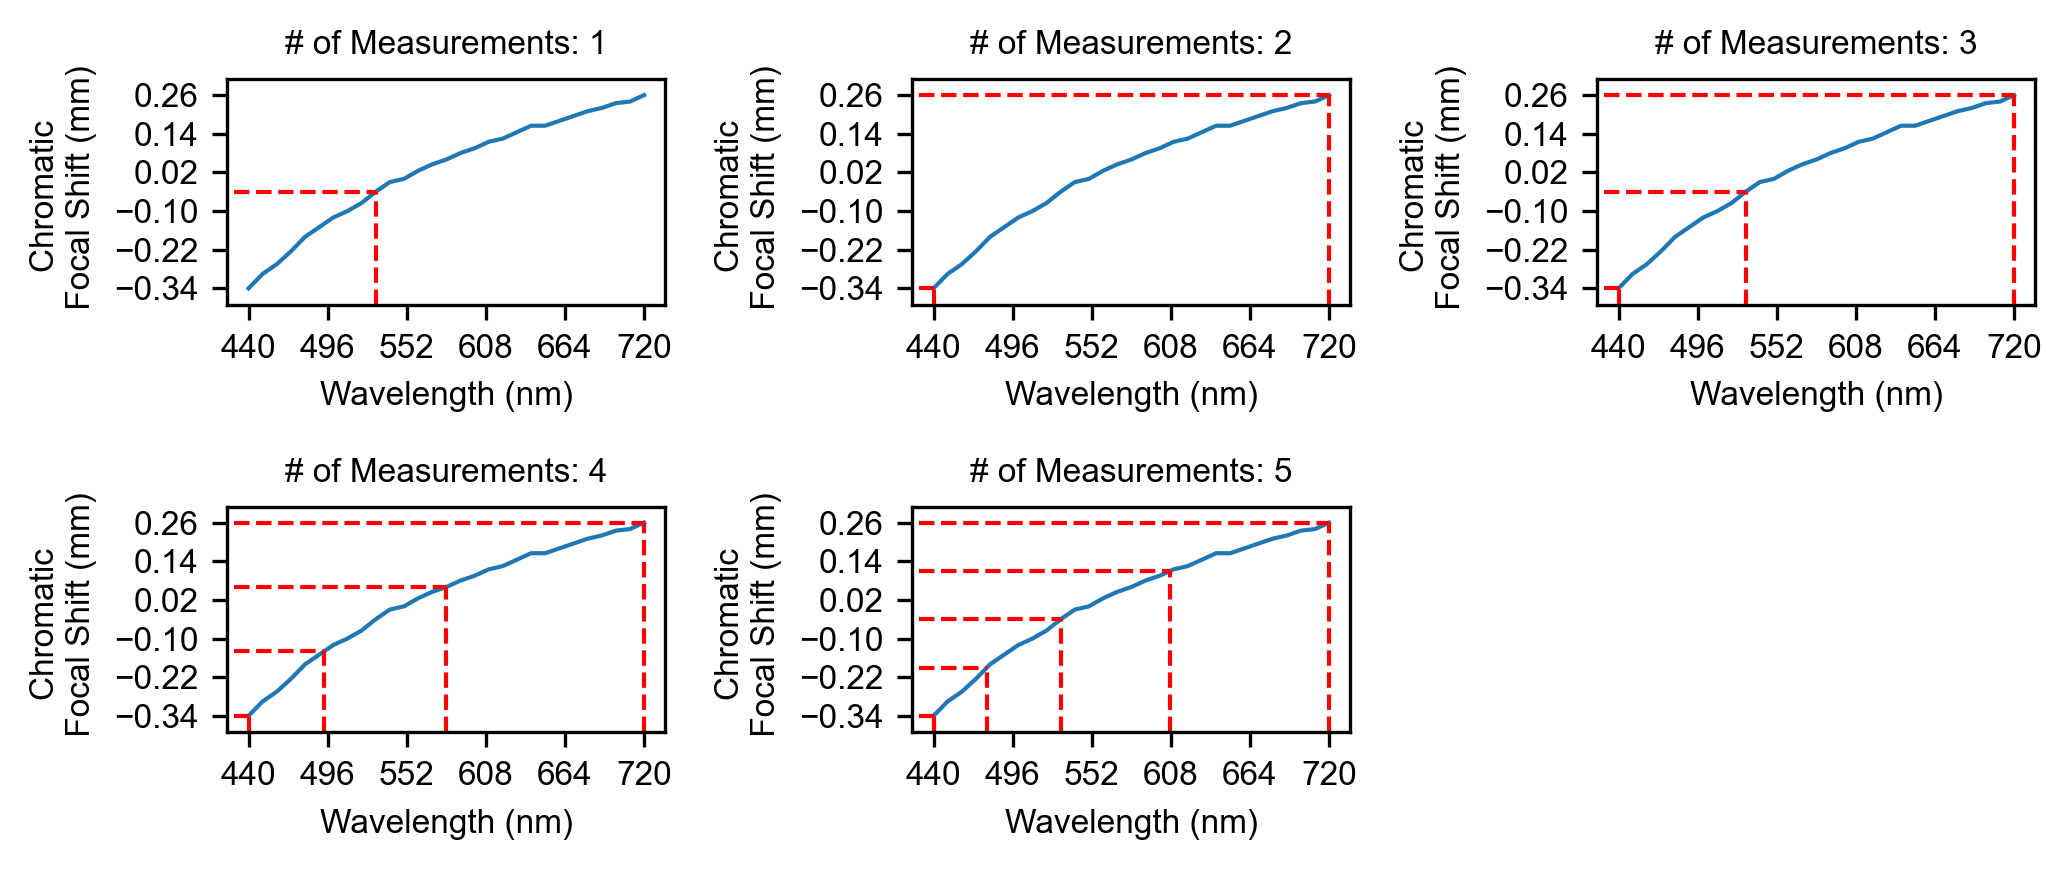}
    \caption{The chromatic focal shifts of different number of measurements.}
    \label{fig:focal_shift_locs}
\end{suppfigure*}

\stepcounter{si}
\section{ADMM Derivation} %S9
\label{sec:supp admm_derivation}
To derive the ADMM, we first formulate the augmented Lagrangian $\mathcal{L}(\bv, \bz, \bu, \boldsymbol{\xi}, \boldsymbol{\eta})$ as:
\begin{equation}
\begin{aligned}
    \mathcal{L}(\bv, \bz, \bu, \boldsymbol{\xi}, \boldsymbol{\eta})=& \frac{1}{2}\| \by - \bC\bv \|_2^2 + \Phi_{\boldsymbol{\theta}} (\bu) + \\
    & \frac{1}{2}\mu_1\| \bv - \hat{\bH}\bz \|_2^2 + \boldsymbol{\xi}^T ( \bv - \hat{\bH}\bz ) + \\
    & \frac{1}{2} \mu_2\| \bu - \bz \|_2^2 + \boldsymbol{\eta}^T ( \bu - \bz ).
\end{aligned}
\end{equation}
In the derivation of the ADMM, the algorithm alternates between solving subproblems for the primary variables and updating the dual variables based on optimality conditions.
More specifically, the updating will be:

\begin{align}
&\bv_{i+1} = \argmin{\bv} \mathcal{L}(\bz_i,\bu_i,\bv,\bxi_i,\beeta_i) \label{eq:v_update}\\
&\bz_{i+1} = \argmin{\bz} \mathcal{L}(\bz,\bu_i,\bv_{i+1},\bxi_i,\beeta_i) \label{eq:x_update}\\
&\bu_{i+1} = \bP^T \phi_{\boldsymbol{\theta}}(\bP(\bz_{i+1} + \boldsymbol{\eta}_i) \\
& \\
&\bxi_{i+1} \leftarrow \bxi_i + \mu_1 ( \bv_{i+1} - \hat{\bH}\bz_{i+1} ) \\
&\beeta_{i+1} \leftarrow \beeta_i + \mu_2 ( \bu_{i+1} - \bz_{i+1}).
\end{align}
In the $\bv$ update, we solve the subproblem \cref{eq:v_update} by using the analytical solution,
\begin{align} \label{eq:analytical_v_update}
    \bv_{i+1} = (\bC^\bT\bC + \mu_1 \bI)^{-1} (\bC^T\by + \mu_1 \hat{\bH}\bz_i - \bxi_i).
\end{align}
In the $\bz$ update, we use the following analytical solution to the subproblem \cref{eq:x_update}:
\begin{equation} \label{eq:analytical_z_update}
\begin{aligned}
    \bz_{i+1} = &(\mu_1 \hat{\bH}^T\hat{\bH} + \mu_2 \bI)^{-1}  \\
    &\quad\left(\hat{\bH}^T(\mu_1 \bv_{i+1} + \bxi_i) + (\beeta_i + \mu_2 \bu_i)\right).
\end{aligned}
\end{equation}

\stepcounter{si}
\section{Prior Information} %S11
\label{sec:prior information}
The choice of prior plays a critical role in determining the quality of reconstruction.
In our experiments, a deep denoiser consistently outperforms the traditional $\ell_1$-norm regularization in handling noise and reconstruction artifacts.
The deep denoiser’s ability to model complex data distributions allows it to effectively suppress noise while preserving fine details in the reconstructed images, without requiring extensive parameter tuning.
This makes it particularly well-suited for scenarios with varying noise levels, as shown in \cref{fig:ablation_reg}.
In contrast, $\ell_1$-norm regularization exhibits a trade-off that depends heavily on the noise level and hyperparameter selection.
When applied conservatively, $\ell_1$-norm regularization performs well in low-noise scenarios, recovering fine details. 
However, it tends to amplify noise when applied to low-SNR measurements, leading to degraded reconstructions.

\begin{suppfigure}[hb!]
    \centering
    \includegraphics[width=\columnwidth]{figs/supp/ablation_regularization.png}
    \caption{\textbf{Effect of prior on reconstruction results} Deep denoiser handles noise and reconstruction artifacts better than L1 norm regularization. Here measurement SNR is given with respect to blurred measurements and reconstruction SNR is given with respect to sharp ground truth images.}
    \label{fig:ablation_reg}
\end{suppfigure}

\stepcounter{si}
\section{Algorithm Implementation} %S10
\label{sec:supp algo_implementation}
The matrix inversion in \cref{eq:analytical_v_update} is straightforward to implement because the matrix is diagonal. 
However, the matrix inversion in \cref{eq:analytical_z_update} necessitates a specialized implementation; otherwise, the computational burden becomes prohibitively high for such a large matrix.
Since each submatrix of $\bH$ represents a 2D linear convolution matrix, we implement it using a 2D circulant convolution by padding the input, such that:
\begin{align}
    \bH \bP \bz = \bH_{\text{circ}} \bP_{pad} \bz_{\text{pad}},
\end{align}
where each block of $\bH_{\text{circ}}$ is a square matrix that performs the 2D circulant convolution.
Since most of the following operations and matrices are applied to the padded version of $\bz$, we define $\Tilde{H} := H + K - 1$ and $\Tilde{W} := W + K - 1$ to simplify the notation.
Here $\bP_{\text{pad}}:=\bB^T \otimes \bI_{\TilH\TilW}$ and $\bx_{\text{pad}}$ denotes the padded version of $\bx$.
With this implementation, we can have the following property:
\begin{align} \label{eq:BCCB_property}
    \bH_{circ} = (\bI_N \otimes \bF^H) \begin{bmatrix}
        \boldsymbol{\Sigma}_{1,1} & \dots & \boldsymbol{\Sigma}_{1,C} \\
        \vdots & \ddots & \vdots \\
        \boldsymbol{\Sigma}_{N,1} & \dots & \boldsymbol{\Sigma}_{N,C}
    \end{bmatrix} (\bI_C \otimes \bF),
\end{align}
where $\bF^H$ denotes the conjugate transpose of the 2D discrete Fourier transform (DFT) matrix $\bF$ with the size of $\TilH \TilW$ and $\boldsymbol{\Sigma}_{i,j} \in \mathbb{C}^{\TilH \TilW \times \TilH \TilW}$ denotes a diagonal matrix.
Specifically, the matrix $\bF$ can be expressed as  
\begin{align}  
    \bF = \bF_{1D, \TilW} \otimes \bF_{1D, \TilH},  
\end{align}  
where $\bF_{1D, n}$ represents a one-dimensional discrete Fourier transform (DFT) matrix of size $n$.
Furthermore, it is assumed that the images in each channel are column-stacked.  

By using the property in \cref{eq:BCCB_property}, we have
\begin{equation} \label{eq:PHHP}
\begin{aligned}
    \bP_{pad}^T &\bH_{circ}^T \bH_{circ} \bP_{pad} \\
    &= \bP_{pad}^T (\bI_C \otimes \bF^H) 
        \hat{\boldsymbol{\Sigma}}
    (\bI_C \otimes \bF) \bP_{pad},
\end{aligned}
\end{equation}
where $\hat{\boldsymbol{\Sigma}} \in \mathbb{C}^{\TilH \TilW C \times \TilH \TilW C}$ is defined as
\begin{align}
    \hat{\boldsymbol{\Sigma}}:= 
    \begin{bmatrix}
        \boldsymbol{\Sigma}_{1,1} & \dots & \boldsymbol{\Sigma}_{1,C} \\
        \vdots & \ddots & \vdots \\
        \boldsymbol{\Sigma}_{N,1} & \dots & \boldsymbol{\Sigma}_{N,C}
    \end{bmatrix}^H
    \begin{bmatrix}
        \boldsymbol{\Sigma}_{1,1} & \dots & \boldsymbol{\Sigma}_{1,C} \\
        \vdots & \ddots & \vdots \\
        \boldsymbol{\Sigma}_{N,1} & \dots & \boldsymbol{\Sigma}_{N,C}
    \end{bmatrix}.
\end{align}
It is evident that each block of the matrix $\hat{\boldsymbol{\Sigma}}$ remains diagonal. 
To further leverage the special structure of $\hat{\boldsymbol{\Sigma}}$, we utilize a permutation matrix $\bP_{\pi} \in \mathbb{R}^{\TilH \TilW C \times \TilH \TilW C}$ to transform it into a block diagonal matrix as:
\begin{align} \label{eq:diagonal_mat}
    \bD = \bP_{\pi}^T \hat{\boldsymbol{\Sigma}} \bP_{\pi},
\end{align}
where $\bD$ denotes a block-diagonal matrix, and the elements of the matrix $\bP_{\pi}$ corresponding to the $i^{\text{th}}$ row and the $j^{\text{th}}$ column are defined as:
\begin{align} 
    (\bP_{\pi})_{ij} =
    \begin{cases} 
        1, & \text{if } j = C \bmod(i-1)_{N_p} + \left\lfloor \frac{i-1}{N_p} \right\rfloor + 1, \\
        0, & \text{otherwise}.
    \end{cases}
\end{align}
Here the scalar $N_p$ equals to $\TilH \TilW$.
By combining \cref{eq:diagonal_mat} and \cref{eq:PHHP}, we have
\begin{equation} \label{eq:diagonal_PHHP}
\begin{aligned}
    \bP_{pad}^T &\bH_{circ}^T \bH_{circ} \bP_{pad}  \\
        &= \bP_{pad}^T (\bI \otimes \bF^H) 
        \bP_{\pi} \bD \bP_{\pi}^T
    (\bI \otimes \bF) \bP_{pad} \\
    &= (\bI \otimes \bF^H)  \bP_{pad}^T 
        \bP_{\pi} \bD \bP_{\pi}^T
    \bP_{pad} (\bI \otimes \bF).
\end{aligned}
\end{equation}
The last equality in \cref{eq:diagonal_PHHP} holds due to the property 
$(\bB \otimes \bI)(\bI \otimes \bF^H) = \bB \otimes \bF^H = (\bI \otimes \bF^H)(\bB \otimes \bI)$.
Using \cref{eq:diagonal_PHHP}, the matrix inversion in \cref{eq:analytical_z_update} can be expressed as:
\begin{equation} \label{eq:fast_mat_inverse}
    \begin{aligned}
        (\mu_1 &\hat{\bH}^T\hat{\bH} + \mu_2 \bI)^{-1} \\
        &= (\bI \otimes \bF^H) \bP_{pad}^T 
        \bP_{\pi} (\mu_1 \bD + \mu_2 \bI)^{-1} \bP_{\pi}^T
        \bP_{pad} (\bI \otimes \bF).
    \end{aligned}
\end{equation}
This reformulation in \cref{eq:fast_mat_inverse} allows us to compute the inverse by inverting only the blocks of the block-diagonal matrix $\bD$.
It is worth noting that, in our implementation, the permutation matrix is not explicitly constructed. Instead, we apply the discrete Fourier transform and matrix inversion along different axes.
By leveraging this approach --- applying operations along specific axes and reshaping the data into a 4D cube --- our implementation achieves sub-second compute time.

To handle extreme model mismatch (i.e., off-axis reconstruction in \cref{sec:supp optical_simulation}), we adaptively adjust the number of basis vectors during optimization. After iteration 4, we evaluate the L2 difference between $\bz$ and $\bu$. If this difference exceeds a predefined threshold, we halve the number of used basis vectors (i.e., rows in $\bB$); otherwise, we keep it unchanged. This adaptive mechanism suppresses noise introduced by model mismatch. The initial number of basis vectors is $16$. Additionally, we terminate the optimization early once it reaches iteration 9. Notably, the model-mismatch denoising module is only triggered in extreme cases (i.e., off-axis reconstruction in \cref{sec:supp optical_simulation}). In most scenarios, SfD converges within 4 iterations.

\stepcounter{si}
\section{Parameter Search} %S8
\label{sec:parameter_search}
The performance of the ADMM method is highly sensitive to its parameters, $\mu_1$ and $\mu_2$, which control the balance between data fidelity and regularization.
These parameters must be carefully tuned to achieve optimal reconstruction quality. 
Improper selection of $\mu_1$ and $\mu_2$ can lead to suboptimal convergence, ringing artifacts, increased numerical errors, or oversmoothing of the reconstructed image.

A new set of hyperparameters should be picked when parameters such as image size, FFT size, input SNR and PSF are changed. 
The retuning of parameters is done through a three-step manual grid search. In the first step, we perform a logarithmic search over a wide range of values, testing $\mu_1$ and $\mu_2$ between $10^{-15}$ and $10^{-5}$, incrementing by a factor of 10 at each iteration. This step provides a coarse estimation of the optimal range for each parameter.
In the second step, we perform a linear grid search within the range identified in the first step. This allows us to narrow down the parameter values with greater precision.
Optionally, a final linear grid search can be conducted around the most promising values from step two to fine-tune the parameters.
We provide the code for this process on our GitHub page.
If our method is to be tested on a new dataset, we recommend first tuning the ADMM parameters on a representative sample image from the dataset.

In \cref{tab:admm_params} we list the ADMM parameters used for both simulation and real data. The simulated datasets consist of $1000 \times 1000$ images with 31 spectral channels, while the real prototype data has different resolution and channel count. Accordingly, separate parameter sets were chosen to ensure stable and efficient convergence in each case.

\begin{supptable}[th!]
    \centering
    \caption{\textbf{ADMM Parameters} are kept constant across experiments on the same dataset. To achieve the best performance, algorithm requires retuning for changes such as input SNR, measurement count or FFT window size. Detailed walkthrough to retune the algorithm for a new dataset is provided in our code. For your convenience, already tuned parameters at different noise levels and image sizes are available in experiment configuration files in our codebase.}
    \label{tab:admm_params}
    \begin{adjustbox}{max width=\columnwidth}
    \begin{tabular}{lcc}
        \toprule
        Data Type & $\mu_1$ & $\mu_2$ \\
        \midrule
        Simulation & $1.20\times10^{-8}$ & $1.1\times10^{-13}$ \\
        Real Data & $1.60\times10^{-8}$ & $3.9\times10^{-13}$ \\
        \bottomrule
    \end{tabular}
    \end{adjustbox}
\end{supptable}

\stepcounter{si}
\section{Light Efficiency of Optical Components} %S4
\label{sec:supp light efficency}
To estimate light efficiency, we assign a transmission coefficient to each optical component based on its transmittance.
For systems with a single optical path, the total efficiency is computed as the product of the transmission coefficients along the path.
For KRISM, which has two optical paths, we take the average efficiency of both paths. 
To ensure fairness, we assume that similar components across all methods have identical transmission properties.
Additionally, we assume all systems share an ideal objective lens with the same aperture size.
See \cref{tab:light_eff} for details.

\begin{supptable*}[t]
    \centering
    \caption{Light Efficiency of optical components and methods}
    \label{tab:light_eff}
    \begin{adjustbox}{max width=\textwidth}
    \begin{tabular}{lccccccccccc}
        \toprule
        Optical Component & Light Efficiency & TF & S. Diff.Cam & S. DefocusCam & MST & Choi el al.  & KRISM (Path 1) & KRISM (Path 2) & 2in1 Cams & Zhan et al.  & Ours \\
        \midrule
        Lens & 0.99 & - & - & 2 & 2 & 2 & 5 & 4 & 5 & 4 & 2 \\
        Diffuser & 0.99 & - & 1 & - & - & - & - & - & - & - & - \\
        DOE & 0.95* & - & - & - & - & - & - & - & 1 & - & - \\
        Mirror & 0.99 & - & - & - & - & - & 2 & - & - & - & - \\
        Compound Lens & 0.9 & 1 & - & - & 1 & 1 & - & - & - & - & - \\
        Diffraction Grating & 0.9 & - & - & - & - & - & 1 & 1 & - & - & - \\
        Prism & 0.9 & - & - & - & 2 & 2 & - & - & - & - & - \\
        Liquid Crystal Shutter & 0.9 & - & - & - & - & - & 2 & 2 & - & - & - \\
        Beam Splitter  & 0.9 & - & - & - & - & - & 2 & 2 & - & - & - \\
        Coded Apertures & 0.5 & - & - & - & 1 & 1 & 1 & 1 & - & - & - \\
        Spatial Light Modulator & 0.5 & - & - & - & - & - & 1 & 1 & - & - & - \\
        Narrow Band Spectral Filter & 0.032 & 1 & 1 & 1 & - & - & - & - & - & - & - \\
        RGB Bayer Filter & 0.4 & - & - & - & - & - & - & - & 1 & - & - \\
        Number of Measurements  & 1/N & 31 & 1 & 5 & 1 & 1 & 5 & 5 & 1 & 3 & 5 \\
        Light Efficiency Per Exposure & - & 0.000936 & 0.032 & 0.0063 & 0.36 & 0.36 &\multicolumn{2}{c}{0.028} & 0.36 & 0.32 & 0.196 \\
        Effective Light Efficiency & - & 0.029 & 0.032 & 0.032 & 0.36 & 0.36 & \multicolumn{2}{c}{0.14} & 0.36 & 0.96 & 0.98\\
        \bottomrule
        *: Estimated from fresnel lenses.
    \end{tabular}
    \end{adjustbox}
\end{supptable*}

\stepcounter{si}
\section{Comparison at Shorter Exposure Times} %S5
\label{sec:shorter_exposure}

We extend the comparison in \cref{tab:comparison} to a shorter exposure setting of $2.9$ seconds (see \cref{tab:exposure_times}). Our method ranks first in both PSNR and SSIM, highlighting the significant advantage of capturing nearly all incident light. Notably, spectral reconstruction accuracy (as reflected by SAM) deteriorates substantially as the exposure time decreases, indicating that photon efficiency is a primary factor in hyperspectral imaging performance.

\begin{supptable*}[th!]
    \centering
    \caption{\textbf{Performance on Harvard dataset for 2.9-second exposures}, all other settings as in \cref{tab:comparison}.}
    \begin{adjustbox}{max width=\textwidth}
    \begin{tabular}{lcccccc}
        \toprule
        Exposure Times: & \multicolumn{3}{c}{2.9 s. } & \multicolumn{3}{c}{5.0 s.} \\
        \cmidrule(lr){2-4} \cmidrule(lr){5-7}
        Modality & PSNR (dB) $\uparrow$ & SSIM $\uparrow$ & SAM ($^\circ$) $\downarrow$ & PSNR (dB) $\uparrow$ & SSIM $\uparrow$ & SAM ($^\circ$) $\downarrow$ \\
        \midrule
        TF  & -4.88 & 0.04 & 88.71 & 4.78 & 0.08 & 70.10  \\
        S. Diff.Cam & 12.03 & 0.37 & 40.88 & 15.59 & 0.46 & 34.98 \\
        S. DefocusCam & 14.96 & 0.46 & \textbf{33.21} & 21.17 & 0.61 & 25.11 \\
        MST  & \underline{21.18} & 0.53 & 38.87 & 30.62 & \textbf{0.92} & 9.33 \\
        Choi et al. & 15.97 & 0.41 & 41.84 & 23.97 & 0.68 & 14.85 \\
        KRISM  & 21.12 & 0.58 & \underline{34.38} & \underline{29.40} & 0.91 & \textbf{6.91}  \\
        2in1 Cams & 19.63 & \textbf{0.61} & 41.90 & 29.11 & 0.87 & 8.72 \\
        Zhan et al. & 6.11 & 0.04 & 71.45 & 14.11 & 0.07 & 23.95 \\
        \textbf{Ours} & \textbf{24.10} & \textbf{0.61} & 36.51 & \textbf{30.81} & \textbf{0.92} & \underline{7.35} \\
        \bottomrule
    \end{tabular}
    \end{adjustbox}
    \label{tab:exposure_times}
\end{supptable*}

\begin{suppfigure*}[hb!]
    \centering
    \includegraphics[width=0.95\textwidth]{figs/supp/lctf_zhan_spectral_curves.png}
   \caption{\textbf{Spectral lines for tunable filter (LCTF) and Zhan et al. \cite{zhan2019hyperspectral}} corresponding to \cref{fig:sim_results}c.}
   \label{fig:lctf_zhan_spectral_lines}
\end{suppfigure*}

\stepcounter{si}
\section{Data Collection Details} %S1
\label{sec:hardware prototype details}
We implemented the prototype described in~\cref{subsec:optical system,subsec:system_specifications,tab:components}, and captured several real scenes, with code and data available on our GitHub page. See prototype details in \cref{tab:components}.
All targets were placed 2.8 m from the camera, well within the system’s 34 cm depth of field, to minimize depth defocus.
To further reduce model mismatch, scenes were positioned close to the optical axis, where spherical and lateral aberrations are least pronounced.
Since our algorithm does not explicitly model these aberrations, we center-cropped each image around the target region, ensuring the reconstructions were evaluated under near-ideal optical conditions. 
Each measurement used a 1-second exposure, giving a total of 5 seconds per scene.

As ground truth, we built a second camera using the same LCTFs employed during calibration and the same grayscale sensor as the SfD prototype.
The filter was stepped from $440$–$720$ nm in $10$ nm increments, yielding 29 spectral channels with $10$ nm bandwidth (see \cref{fig:spectral_filter}).
To ensure consistent radiometric response, we imaged a uniform white diffusive object under a broadband tungsten–halogen lamp and applied per-channel gain coefficients so that the surface had constant value 1.0 across all bands.
This calibration compensates for the wavelength-dependent transmission of the filter and the spectral sensitivity of the sensor and other optical components.
Ground-truth exposures took approximate 3 minutes in total, shared by 29 measurements, and used the same scene geometry and illumination as the SfD prototype.
\begin{supptable}[ht]
\caption{
\textbf{Prototype \& calibration components.}
Components used in the prototype system and calibration.
}
\centering
\begin{tabular}{ll}
\hline
\textbf{Component} & \textbf{Series / Model} \\
\hline
Objective lens & Thorlabs LBF254-050-A (Best-form) \\
Focusing lens & Thorlabs AL2550M-A \\
Grayscale sensor & FLIR GS3-U3-23S6M \\
$100$ $\mu$m Pinhole & Thorlabs P100K \\
LCTF & Thorlabs K2VB1 \\
Light source & Tungsten–halogen lamp \\
\hline
\end{tabular}

\label{tab:components}
\end{supptable}

\stepcounter{si}
\section{Optical Aberrations} %S3
\label{sec:supp aberrations} 
In the SfD algorithm, axial chromatic aberration serves as the primary spectral encoding mechanism.
To assess the extent of other aberrations in our prototyped SfD camera, we analyze third-order aberrations using the lens model and CodeV.
As illustrated in \cref{fig:sim_aberrations_simple}, axial chromatic aberration is the dominant aberration, with its combined aberration coefficient being 6.3 times larger than that of spherical aberration ($-0.095$ mm to $-0.015$ mm), and 4 times larger than all other aberrations combined (sum of absolute values $0.024$ mm) . Signed values of each third-order aberration are included for completeness in \cref{fig:sim_aberrations}.

\begin{suppfigure}[ht!]
  \centering
  \includegraphics[width=\columnwidth]{figs/supp/aberration_total.png} 
   \caption{\textbf{Longitudinal Chromatic Aberration dominates.} Our optical design features creates significantly more longitudinal chromatic aberration than any other 3rd order aberrations, ensuring the presence of our method's chromatic signal.}
   \label{fig:sim_aberrations_simple}
\end{suppfigure}

\begin{suppfigure}[h!]
  \centering
  \includegraphics[width=\columnwidth]{figs/supp/aberration_a.png}
   \caption{\textbf{3rd Order Aberrations.} Graph describes the amount of aberration introduced at each surface of the lenses (Each lens has 2 surfaces). The overall effect of the imaging system (``Image Plane") has spherical (SA) aberration co-efficient $-0.015$ mm, and the combined axial (AX) chromatic aberration coefficient is $-0.095$ mm.}
   \label{fig:sim_aberrations}
\end{suppfigure}

\stepcounter{si}
\section{Component Spectral Characteristics} %S2
\label{sec:optical_system}
In \cref{fig:spectral,fig:spectral_filter}, we present the spectral characteristics of the critical components used in the prototype.  
Throughout all experiments, we account for the camera's quantum efficiency.
The data presented in \cref{fig:spectral} is also available on our GitHub page.

\begin{suppfigure}[hb!]
    \centering
    \includegraphics[width=\columnwidth]{figs/supp/spectral.png}
    \caption{\textbf{Component spectral characteristics.} The quantum efficiency of the camera and the transmittance of the filter were obtained from the manufacturer's specifications. }
    \label{fig:spectral}
\end{suppfigure}

\begin{suppfigure}[hb!]
    \centering
    \includegraphics[width=\columnwidth]{figs/supp/LCTF_transmission.png}
    \caption{
    \textbf{Normalized filter transmission spectra.} We show the representative transmission spectra of the used LCTFs. The data is from the manufacturer's specifications.
    }
    \label{fig:spectral_filter}
\end{suppfigure}

\stepcounter{si}
\section{Stacked Measurements} %S14
\label{sec:stacked measurements}
To better understand the functionality of our camera and verify whether our measurements contain color information, we conducted a visualization experiment.
We stacked three grayscale measurements, corresponding to in-focus wavelengths of 671 nm, 546 nm, and 442 nm ($z_3$, $z_7$, and $z_{11}$), along the channel dimension.
Finally, we white balanced the images using the white patch in the color checker.
As shown in \cref{fig:ablation_stacked_meas} and \cref{fig:wb_ablation_stacked_meas}, optical system recovers some color just by dispersing the power of out of focus wavelengths without any computation.

\begin{suppfigure}[hb!]
    \centering
    \includegraphics[width=\columnwidth]{figs/supp/ablation_stacked_meas.png}
    \caption{\textbf{RGB Scene Images Composed Using Measurements without White Balance} The four scene images are composed by stacking three measurements, corresponding to in-focus wavelengths of 671 nm, 546 nm, and 442 nm, which associated to $z_3$, $z_7$, and $z_{11}$.}
    \label{fig:ablation_stacked_meas}
\end{suppfigure}

\begin{suppfigure}[hb!]
    \centering
    \includegraphics[width=\columnwidth]{figs/supp/wb_meas_compose.png}
    \caption{\textbf{RGB Scene Images Composed Using Measurements with White Balance} The four scene images are generated by combining three measurements, each corresponding to specific in-focus wavelengths: 671 nm, 546 nm, and 442 nm, which associated to $z_3$, $z_7$, and $z_{11}$. White balance adjustments are applied to ensure accurate color representation. The reference white color is taken from the white square of the color-chart scene image.}
    \label{fig:wb_ablation_stacked_meas}
\end{suppfigure}

\stepcounter{si}
\section{Chromatic Focal Shift} %S6
\label{sec:chromatic_focal_shift}

Simulated and measured chromatic focal shift of our lens pair is given in \cref{fig:chromatic_focal_shift}.
Chromatic focal shift line determines how the size of PSF will change across wavelengths.
Our measurements confirm the expected trend and allow us to correct for non-idealities in the real system.

\begin{suppfigure}[ht!]
    \centering
    \includegraphics[width=\columnwidth]{figs/supp/chromatic_focal_shift.png}
    \caption{\textbf{Chromatic focal shift.} The focal length change is obtained by the combined focal length formula, $\frac{1}{f}=\frac{1}{f_1}+\frac{1}{f_2}-\frac{d}{f_1 f_2}$, where $f$, $f_1$, $f_2$, and $d$ are an effective focal length, focal lengths of the lens pair in our optical system, and the distance between the two lenses, respectively. For simulation we use CodeV Analysis Toolbox}
    \label{fig:chromatic_focal_shift}
\end{suppfigure}

\stepcounter{si}
\section{Reconstruction using different number of measurements} %S13
\label{sec:supp recon diff meas}
In addition to evaluating the spectral accuracy of the reconstruction using SAM as the number of measurements increases (see \cref{fig:trends}), we also assess the reconstruction accuracy through RGB visualization as shown in \cref{fig:rgb from measurements}.
\begin{suppfigure*}[hb!]
    \centering
    \includegraphics[width=\textwidth]{figs/supp/num_meas.png}
    \captionsetup{justification=centering, width=\textwidth}
    \caption{\textbf{Reconstruction Quality Improves with Measurement Count.} The inclusion of additional measurements stabilizes the inversion and produces less spatial artifacts and higher quality spectra(see \cref{fig:trends}). Unlike our simulated benchmarks, in the real data case each additional measurement adds linearly to the total exposure time. See \cref{fig:focal_shift_locs} for the corresponding lens locations.
    }
    \label{fig:rgb from measurements}
\end{suppfigure*}

\stepcounter{si}
\section{Depth of Field Analysis} %S7
\label{sec:supp dof}
With SfD, the PSF size is used as a cue to recover the spectrum. 
However, our algorithm does not account for PSF size changes caused by depth variations in the scene.
The theoretical depth of field (DoF) of our optical system ($s \gg f$) is given by:
\begin{equation}
\begin{aligned}
    & \text{DoF} \approx \frac{2NCs^2}{f^2},
\end{aligned}
\end{equation}
where $N$ is the aperture number, $C$ is the circle of confusion, $s$ is the distance between the camera and the subject, and $f$ is the effective focal length of the system.
At a depth of $2.8$ m and a circle of confusion size of approximately 2 pixels (11.76 $\mu$m), our system has a DoF of $0.34$ m. 
In simulations, we assume the scene is flat and has a depth of $2.8$ m.
For real experiments, we ensured that all test targets were positioned within this region to minimize the effects of depth variations on PSF size.

We further confirm our depth range with our hardware prototype as shown in \cref{fig:trends}. The reconstruction results used in \cref{fig:trends} are presented in \cref{fig:depth_test}.

\begin{suppfigure}[hb!]
    \centering
    \includegraphics[width=\columnwidth]{figs/supp/depth_test.png}
    \caption{\textbf{Color checker reconstruction at varying depth (distance from camera).} We collected focal stacks at different depths. For each depth, we used the same scene (i.e., identical target and illumination) and acquired five grayscale measurements for hyperspectral reconstruction. Our method maintains similar reconstruction quality even when the theoretical depth assumption (2.64–2.98 m) is mildly violated. Brightness boosting was applied for visualization (10\% for the top row and 70\% for the bottom row).}
    \label{fig:depth_test}
\end{suppfigure}

\stepcounter{si}
\section{Field of View and Off-axis Reconstructions} %S12
\label{sec:supp optical_simulation}

To reconstruct the spectral image, we assume that the point spread function (PSF) is shift-invariant across the field of view.
However, in practice, the PSF exhibits spatial variation due to optical aberrations.
In particular, our aspherical focusing lens effectively suppresses spherical aberration near the optical axis, but this comes at the cost of aspherical aberrations, which become more pronounced at larger field angles.
Despite this, we can approximate shift invariance within the center of the image (the area close to optical axis), and solve the problem accordingly.
For the scenes presented in this paper, we empirically validate that our model successfully reconstructs spectral information within a $10^\circ$ field of view ($-5^\circ$ to $5^\circ$ from the optical axis).

To evaluate the feasibility of patch-based reconstruction, we repeated the calibration process with the point light source positioned at a $15^\circ$ field angle.
We then captured a focal stack from an object at the same location.
As shown in \cref{fig:off_axis_psf}, although the measured PSFs closely match simulations, our reconstruction algorithm fails to converge outputting the result shown in \cref{fig:off_axis_recon}.
This suggests that our optical forward model does not fully account for aberrations at larger field angles, leading to significant model mismatch.
Extending field of view through patch-based reconstruction remains an open challenge for future work.

\begin{suppfigure}[ht!]
  \centering
  \includegraphics[width=\columnwidth]{figs/supp/PSF_Grid.png}
   \caption{\textbf{Comparison of PSFs at different conditions.} We validate our PSFs using CodeV at standart settings, with a large depth of field error, and at a large field angle that is outside our working FOV range.}
   \label{fig:off_axis_psf}
\end{suppfigure}

\begin{suppfigure}[ht!]
  \centering
  \includegraphics{figs/supp/off_axis_and_3x.png}
   \caption{\textbf{Off-axis reconstruction failure.} Even when using the corresponding off-axis filter stack shown in \cref{fig:off_axis_psf}, the reconstruction of a color checker at 15$^\circ$ off-axis fails. Shown here at the original brightness (top) and 3$\times$ brightness (bottom), the results are noisy and monochromatic, because our algorithm iteratively reduces its representation dimension to reach convergence (see \cref{sec:supp algo_implementation}). Our optical system provides aberrations that enable SOTA hyperspectral performance for the standard paraxial field of view, but future work is needed to extend its performance at large field angles.}
   \label{fig:off_axis_recon}
\end{suppfigure}

\begin{suppfigure*}[hb!]
    \centering
    \includegraphics[width=0.95\textwidth]{figs/per_channel/minion_combined_channels.png}
    \caption{\textbf{Full reconstruction of minion scene.} Per-channel images (top: ground truth, bottom: reconstruction). See per-channel labels for central wavelength and reconstruction PSNR.}
   \label{fig:fullrecon_mi}
\end{suppfigure*}

\begin{suppfigure*}[hb!]
    \centering
    \includegraphics[width=0.95\textwidth]{figs/per_channel/color_checker_combined_channels.png}
   \caption{\textbf{Full reconstruction of Noah scene.} Per-channel images (top: ground truth, bottom: reconstruction). See per-channel labels for central wavelength and reconstruction PSNR.}
   \label{fig:fullrecon_colorchecker}
\end{suppfigure*}

\begin{suppfigure*}[hb!]
    \centering
    \includegraphics[width=0.95\textwidth]{figs/per_channel/noah_combined_channels.png}
    \caption{\textbf{Full reconstruction of Noah scene.} Per-channel images (left: ground truth, right: reconstruction). See per-channel labels for central wavelength and reconstruction PSNR.}
   \label{fig:fullrecon_noah}
\end{suppfigure*}

\begin{suppfigure*}[hb!]
    \centering
    \includegraphics[width=0.95\textwidth]{figs/per_channel/resolution_target_combined_channels.png}
   \caption{\textbf{Full reconstruction of pinwheel scene.} Per-channel images (left: ground truth, right: reconstruction). See per-channel labels for central wavelength and reconstruction PSNR.}
   \label{fig:fullrecon_pinwheel}
\end{suppfigure*}

\begin{suppfigure*}[hb!]
    \centering
    \includegraphics[width=0.95\textwidth]{figs/per_channel/book_combined_channels.png}
    \caption{\textbf{Full reconstruction of book scene.} Per-channel images (left: ground truth, right: reconstruction). See per-channel labels for central wavelength and reconstruction PSNR.}
   \label{fig:fullrecon_book}
\end{suppfigure*}
